# Supplementary material for: ST-Adapter: Parameter-Efficient Image-to-Video Transfer Learning
Source: arXiv:2206.13559 source file (2022-10-13)
Supplement: Supplementary file 1 [file new_baseline.tex]

% \begin{table}[h]
%     \centering
%     \caption{{\bf Comparison with two additional baselines.} The {\it TM?} column indicates whether the method uses temporal modeling, {\it i.e.}, a temporal aggregation method other than average pooling. For other details see Table 1 in the main manuscript.}
%     \begin{tabular}{ll|cc|cc|cc}
%     \toprule
%      & & & & \multicolumn{2}{c|}{CLIP} & \multicolumn{2}{c}{ImageNet-21K} \\
%     \cmidrule{5-8}
%     \begin{tabular}{c}Fine-tuning\\Methods\end{tabular} & Architecture &
%     TM? &
%     \begin{tabular}{c}Fine-tuned\\Params (M)\end{tabular} & K400 & SSv2 & K400 & SSv2 \\
%     \midrule
%     Full Fine-tuning w/ ST-Adapter & SA + TA & \cmark & 93.31 & 82.3 & 66.3 & - & - \\
%     \midrule
%     BitFit \cite{bitfit} & SA & & 0.41 & 77.6 & 33.6 & 71.1 & 27.2 \\
%     \midrule
%     ST-Adapter (Ours) & SA & \cmark & 7.20 & \textbf{82.0} & \textbf{65.6} & \textbf{76.5} & \textbf{62.8}\\
%     \bottomrule
%     \end{tabular}% <------ Don't forget this %
%     \label{tab:new_baseline}
% \end{table}

\begin{table}[h]
    \centering
    \caption{{\bf Comparison with two additional baselines.} The {\it TM?} column indicates whether the method uses temporal modeling, {\it i.e.}, a temporal aggregation method other than average pooling. For other details see Table 1 in the main manuscript.}
    \begin{tabular}{ll|cc|cc}
    \toprule
    \begin{tabular}{c}Fine-tuning\\Methods\end{tabular} & Architecture &
    TM? &
    \begin{tabular}{c}Fine-tuned\\Params (M)\end{tabular} & K400 & SSv2 \\
    \midrule
    \revision{Full Fine-tuning w/ ST-Adapter} & \revision{SA + TA} & \revision{\cmark} & \revision{93.31} & \revision{82.3} & \revision{67.3} \\
    \midrule
    BitFit \cite{bitfit} & SA & & 0.41 & 77.6 & 33.6 \\
    \revision{Adapter \cite{adapter}} & \revision{SA} & & \revision{6.77} & \revision{81.6} & \revision{46.2} \\
    \midrule
    ST-Adapter (Ours) & SA & \cmark & 7.20 & 82.0 & 66.3 \\
    \bottomrule
    \end{tabular}% <------ Don't forget this %
    \label{tab:new_baseline}
\end{table}
