# Supplementary material for: ST-Adapter: Parameter-Efficient Image-to-Video Transfer Learning
Source: arXiv:2206.13559 source file (2022-10-13)
Supplement: Supplementary file 2 [file epic.tex]

\begin{table}[h]
    \centering
    \caption{\textbf{Comparing the state-of-the-art video recognition methods on Epic-Kitchens-100}}
    \begin{tabular}{l|c|c|cc}
        \toprule
        Method & Pre-train data & \#Frames & Verb & Noun \\
        \midrule
        ViViT-L \cite{vivit} & IN21K+K400 & 16 $\times$ 3 $\times$ 10 & 66.4 & 56.8 \\
        MFormer-B \cite{mformer} & IN21K+K400 & 16 $\times$ 3 $\times$ 10 & 66.7 & 56.5 \\
        XViT(8x) \cite{xvit} & IN21K+K400 & 8 $\times$ 3 $\times$ 1 & 66.7 & 53.3 \\
        \midrule
        ViT-B/16 w/o ST-Adapter (Full Fine-tuning) & CLIP & 8 $\times$ 3 $\times$ 1 & 54.8 & 50.4 \\
        ViT-B/16 w/ ST-Adapter (Ours) & CLIP & 8 $\times$ 3 $\times$ 1 & 67.6 & 55.0 \\
        \bottomrule
    \end{tabular}
    \label{tab:epic}
\end{table}
