# Supplementary material for: ST-Adapter: Parameter-Efficient Image-to-Video Transfer Learning
Source: arXiv:2206.13559 source file (2022-10-13)
Supplement: Supplementary file 3 [file kernel_shape.tex]

% \begin{table}[h]
%     \centering
%     \caption{\textbf{Effects of kernel shape.}}
%     \begin{tabular}{cccc}
%         \toprule
%         Kernel Type & Kernel Size & K400 & SSv2 \\
%         \midrule
%         Local & $1 \times 1 \times 1$ & 81.6 & 46.2 \\
%         Spatial & $1 \times 3 \times 3$ & 81.4 & 46.2 \\
%         Temporal & $3 \times 1 \times 1$ & \textbf{82.0} & \textbf{66.2} \\
%         Spatio-temporal & $3 \times 3 \times 3$ & \textbf{82.0} & 65.6 \\
%         \bottomrule
%     \end{tabular}
%     \label{tab:kernel_shape}
% \end{table}

\begin{table}[h]
    \centering
    \caption{\textbf{Effects of kernel shape.} Kernel size is denoted as $k_T \times k_H \times k_W$ for temporal, height and width sizes.}
    \begin{tabular}{ccc}
        \toprule
        Kernel Size & K400 & SSv2 \\
        \midrule
        $1 \times 1 \times 1$ & 81.6 & 46.2 \\
        $1 \times 3 \times 3$ & 81.4 & 46.2 \\
        $3 \times 1 \times 1$ & \textbf{82.0} & \textbf{66.2} \\
        $3 \times 3 \times 3$ & \textbf{82.0} & 65.6 \\
        \bottomrule
    \end{tabular}
    \label{tab:kernel_shape}
\end{table}
