# Supplementary material for: ST-Adapter: Parameter-Efficient Image-to-Video Transfer Learning
Source: arXiv:2206.13559 source file (2022-10-13)
Supplement: Supplementary file 4 [file training_time.tex]

\begin{table}[h]
    \centering
    \caption{\textbf{Training time and memory.}}
    \begin{tabular}{l|c|c}
        \toprule
        Model & 
        \begin{tabular}{c}Training GPU-hours \\(K400)\end{tabular} & \begin{tabular}{c}Peak mem \\ (M)\end{tabular} \\
        \midrule
        TimeSformer\cite{timesformer} (Full Fine-tune)	&60 (+161\%)	& 21694 (+52\%) \\
        ViT-B/16 (Full Fine-tune)	&40 (+74\%)	&17275 (+21\%) \\
        ViT-B/16 w/ ST-Adapter	&23	&14238 \\
        \bottomrule
    \end{tabular}
    \label{tab:train_time}
\end{table}
